# Supplementary material for: Observation of the decay $\Lambda^0_b \to p K^- \mu^+ \mu^-$ and a search for $C\!P$ violation
Source: arXiv:1703.00256 source file (2018-04-15)
Supplement: Supplementary file 1 [file supplementary.tex]

\section*{Supplementary material for LHCb-PAPER-2016-059}
\begin{figure}[h]
\centering
\includegraphics[scale=0.45]{figs/mX_eff.pdf}
\captionof{figure}{Background-subtracted and efficiency-corrected $m(pK^{-})$ distribution for the decay \LK.}
\end{figure}
\begin{figure}[h]
\centering
\includegraphics[scale=0.45]{figs/chi_eff.pdf}
\captionof{figure}{Background-subtracted and efficiency-corrected distribution of the angle $\chi$ for the decay \LK.}
\end{figure}
